# Supplementary material for: Why did I fail? A Causal-based Method to Find Explanations for Robot Failures
Source: arXiv:2204.04483 source file (2022-06-21)
Supplement: Supplementary file 1 [file AdditionalText.tex]

\textcolor{blue}{
Discussion on what to do if the causal graph learning is incorrect (collected some quotes from~\cite{Sharma21}. 
)
\begin{itemize}
    \item Given observed data, causal inference is the process of using domain assumptions to estimate the effect of a desired action. 
    \item Formally, a causal effect is always defined w.r.t. a causal model that encodes assumptions that typically cannot be learned from observed data.
    \item In practice, obtaining plausible assumptions to develop the causal graph either by human experts or by causal discovery algorithms is potentially the biggest challenge of doing causal analysis and that is often overlooked.
    \item Every causal estimate depends on assumptions that cannot be fully tested from observed data. Importantly assumptions does not wash out even with infinite data. 
    \item In general, it is difficult to judge the quality of any obtained causal estimate from observed data, since the "correct" causal effect depends on the modelling assumptions. 
    \item While causal graphs provide a formal abstraction for expressing causal assumptions, no such well-accepted method exists for validating those assumptions. Most works focus on sensitivity analyses that describe how an obtained estimate changes if we change any of the identifying assumptions.
    \item First type of methods is similar to cross-validation loss metric:  However, in the absence of ground-truth data with the true causal effects, and in the absence of experimental data from a randomized-controlled trial, these methods use secondary estimators to estimate auxiliary predictive models that are being used in the quality metrics.Second type of methods, construct a new, simulated data-set where the full data-generating process (DPG) is known and hence the ground-truth causal effect is also known. 
    \item Possible solutions: Machine teaching methods (human-in-the-loop); Expressing assumptions as constraints, High-level causal graphs, sufficient partial graphs
\end{itemize}
Detecting directions of causal effects is not always possible just from data~\cite{Peters17}. Crucial question: is the structure identifiable from the joint distribution? In general: no!!!! E..g consider the very simple case of only two variables. There are some tricks/assumptions on the data which would allow algorithms to direct edges:
\begin{itemize}
    \item 
\end{itemize}}

\subsection{Discuss conditional probabilities vs. interventional probabilities}
\textcolor{blue}{An interesting distinction between the two examples is the possibility of interventional data and the question if we actually want interventional probabilities. For the failure explanation we might get the outcome that the container has been too small and not high enough. If we calculated the interventional probability, with interventions given the suggested variable parametrization, we would decouple the influence of container type to the height and size. In other words, we would assume the object stays the same, but we would simply change size and height independently from each other.
However, size and height of a container is influenced by the type of the container, and additionally depend on each other (e.g., the larger the bowl, the higher it is), so, in practice, if we need to change the size of the container we might also need to change the object itself, e.g. take a plate instead of a bowl. Thus, the question arises if we should take interventional or conditional probabilities, for failure prediction. In the particular case of dropping a sphere into a container, we opted for taking the conditional probabilites. In the example of cube stacking, conditional probabilities are equal to interventional probabilities, since xoff, yOff and dropOff do not have any parent variables.}

\textcolor{blue}{
Comparison
\begin{itemize}
    \item probabilistic(yes/no) 
    
\end{itemize}}

\textcolor{blue}{
Comparing two methods with respect to our usecases (stacking cube and dropping objects):
\textbf{Explainable AI fpr Robot Failures: Generating Explanations that improve user assistance in Fault Recovery:
\begin{itemize}
    \item Most existing techniques target domain experts
    \item Explain cause of an unexpected failure during an agent's plan execution to non-experts
    \item what types of information within a set of hand-scripted explanations are most helpful to non-experts for failure and solution identification
    \item autonomous generation of failure explanations
    \item context and history
    \item Introducing error explanations designed to explain failures that occur during the execution of a task
    \item encoder-decoder model for autonomously generating natural language explanations to generate context0based history explanations within a continuous state-space
    \item internal vs. external errors: System vs. Environmental failures.
\end{itemize}}}
Possible categories:
\begin{itemize}
    \item generation of failure descriptions
    \item Representative sample of failures in robot behavior (fault-tree analysis): 
    \begin{itemize}
        \item Failure Type: Navigation, Arm Motion Planning, Object Detection
        \item Failure Cause: Mislocalization, Controller Error, Obj. too far away, Obj. too close to others, obj not present, Obj. occluded
        \item Failed Action: segment, move, grasp, detect
        \item Failure Resolution: Look around till relocalized, recalibrate motors, reposition closer to obj., move other obj. further away, find obj. at another location, move other obj. until unoccluded
    \end{itemize}
    \item only one possible cause
    \item Input: (both for learning and for applying)
    \item Output: (both for learning and for applying)
    \item Level of failure abstraction
    \item State space
\end{itemize}
Recall that the agent's state space is defined as $S=S_e \cap S_l \cap S_i \cap S_k$. We derice the features, $U = X \cup N \cup o$ for the encoder-decoder model from S. The object of interest , $o \in S_e$, is specified as part of the task and represetned by its word embedding in U. The environment, X, is comprised of the word embeddings of the names of the objects, $Obj_G$, located in the robot's are of interest. The remaining continuous features characterise the robot and the target object in the environment. 

Basically what we discuss in this section, how two other approaches which are very relevent/related to our proposed approach, and discuss differences in terms of several categories.
\begin{itemize}
    \item Failure representation (Fault trees + encoder-decoder network): Failure causes are presented within the framework of \textit{Fault Trees}. Fault trees break down a failure into Failure types (like Navigation, arm motion planning or object detection), which each can have several potential failure causes (e.g. mislocilization or controller error) and can occur during an action like move, segment or grasp  
    \item State Space + encoder-decoder input: basically object/robot positions, but not features like object size. E.g. stacking failed because 
    \item Output: language representation of the failure vs. contrastive variables (which would definetly profit from being encoded in form of language).
    \item (Model learning) Learning the encoder-decoder model: Provide enough simulations of the robot performing the two tasks of   
    \item Largest difference: In some sense errors are again encoded in a black-box. E.g., understanding like 'why did a stacking fail and which variables are relevant for that error', are encoded in a encoder-decoder structure. In order to get this level of explanations, we could define them specifically as failure causes $F_C$, but then we could not profit from the more flexible capabilites of the causal BN. 
\end{itemize}

\textbf{Probabilistic Effect Prediction through Semantic Augmentation and Physical Simulation}

Contributions:
\begin{itemize}
    \item probabilistic extension to the concept of action templates
    \item framework to derive probabilities from little experience and physical simulation that generalizes to abstract object classes
    \item adaptation of a probabilistic symbolic planner to optimize a sequence of real world robot actions w.r.t. success probabilities
    \item Baseline approach vs. updating effect probabilities online (ML?) vs. Refining Predictions with Physical Simulation; Beta distribution
\end{itemize}

Possible categories:
\begin{itemize}
    \item Probabilistic action representation (or action representation in general)
    \item generalization (e.g. through BN vs. through ontology) How does the previous method generalize?
    \item What kind of manual inputs do we need (e.g. deinfe probabilistic action templates vs. goal definition in our case + variable definition vs. Failure tree.) 
\end{itemize}

\begin{itemize}
    \item our framework captures autonomously the semantic information in a scene to produce semantically descriptive explanations for everyday users.
    \item To generate failure=focused explanations that are semantically grounded, we leverage both smenatic scene graphs to extract spatial relations and object attributes from an environment, as well as pairwise ranking. 
    \item natural language explanations are effective in improving user confidence in an AI system, and in improving user confidence in fault recovery
    \item a contributing factor is the ability to incorporate situational or environmental context from an agent's environment. 
    \item require all domain specific contexts to be hand=annotated a priori preventing generalizability
    \item How can we autonomously extract contectual information grounded in an environment to provide meaningful explanations of system failures to everyday users?
    \item key innovation: use a scene graph to produce semantically descriptive explanations that communicate why a failure to manipulate a given object in the scene occurred. 
    \item pairwise ranking to produce semantically descriptive explanations. Pairwise ranking can be utilizied to autinomously place attention on parts of a scene graph output that are relevant to a given failure. 
    \item We observed, that for all failure types, the semantically descriptive explanations are perceived as significantly more useful than no explanations and the CB explanations.
    \item explanations grounded in inter-object relationsships and object attributes
    \item We adapt thet state-of-the-art scene graph model MOTIFNET to predict spatial relationsships and object attributes in a given scene
    \item We observe that SSG explanations are more semantically richer adn detailed than their CB counterparts. However, we also observe that these explanations include extraneous, semantic information that hides the true cause of a failure. 
    \item Pairwise ranking is used to learn preferences between pairs of entities when multiple available entities exist. 
    \item semantic scenegraph provides spatial information (close to, far away, occluded) as well as object attributes (like heavy, large, hazardous, slippery, fragile etc.)
    \item They yse a random forest classifier, trained using cross validation vis scikit-learn. Depending on the predicted label, the rank of one or both relationshups is incremented (lines 5-10). The resulting lost of relationships L, sorte by rank is returned. Not, annotation of a training label 0, 1, or 2 is determined via domain knowledge of the failure scenario.
\end{itemize}
To develop SSG explanations, we follow a template-based approach that traverses a scene graph, G, and extracts a subgraph g containing all relations rk which contain dobj as a nod ein the triple. To generate an SSG expalantino, we drescribe g, the elements of the scene that pertain to our object of interest. Specifically, we format the explaantion as The robot could not pick up the dobj because reasoning, where reasoning is a list of phrases that enumerates all the object relations. In every scene, the SSG explanations include all relationsshiups associated with dobj. We observe that SSG explaantions are more semantically richer and detailed than their CB counterpart. In addition to extracting a subgraph g, we utilize pairwise ranking to autonomously determine the relevancy of each truple r in g.

\textcolor{blue}{It is not easy to plot the dropping success probability conditional on all its parents at the same time, since this would require a four-dimensional plot. However, we plot the success chance with respect to \texttt{xOff}, \texttt{yOff} and \texttt{ContainerSize} (Fig.~\ref{fig:stackSucc2}), with respect to \texttt{xOff}, \texttt{yOff} and \texttt{ContainerHeight} (Fig.~\ref{fig:stackSucc3}) and also investigate how likely the dropping will succeed for each \texttt{ContainerType} (Fig.~\ref{fig:stackSucc4}). Fig.~\ref{fig:stackSucc2} indicates, that larger sized objects are more tolerant to x/y-offsets (rightmost subplot) compared to small sized objects (leftmost subplot). However, if we only consider the container hight, we cannot see the same trend. The interesting part is that the intervals with least and most height (h1, h5) are only inhabited by plates and cups respectively. Plates are only represented in intervals h1 and h2, and cups are spread among the intervals h2-h4. The dropping success in h5 is solely based on glasses, however, glasses, in general do not have such a large dropping success probability in the chosen intervals, in particular for more extreme x/y-offsets, due to the limited diameter of the glasses (Fig.~\ref{fig:stackSucc4}). The dropping success in intervals h2-h4 is mainly due to the bowl. Bowls, in general, were found to have the highest success when it comes to catching dropped spheres (Fig.~\ref{fig:stackSucc4}). Since bowls have a wide diameter, the success at the most extreme x/y-intervals increases. The larges ares of success can be found, however in interval h2, which covers all the large plates. We conclude, that the physical processes of the sphere dropping experiment are again well reflected in the obtained conditional probability table, which was analyzed in this section, but again, would like to point out that there might be a sim2real gap, since some parameters like the bounciness depends also on the chosen material of the objects. }

\textcolor{blue}{Our approach of explaining action failures combines the area of learning task execution models with the generation of explanations when the task executions fail. In this section, we therefore compare our method with two baseline approaches, one from the area of execution model learning~\cite{Bauer20ICRA}, and two from the area of explanation generation~\cite{Das21, Das21b}, with respect to the two presented usecases of stacking cubes and dropping spheres in containers. Generally there are many reasons for failures and the two works of~\cite{Das21, Das21b} tackle two possible explanation models (e.g., the context based history and environment relations) but they are not capable of capturing the context depend continuous variables that cause errors in the two experiment cases.}

\textcolor{blue}{\cite{Bauer20ICRA} present an approach to learn probabilistic action models which are based on action templates. Action templates describe the preconditions and effects of an action in form of high-level planning operators. The authors assume that the action templates, in particular the choices of preconditions and effects have been predefined by an expert. Our approach is less restrictive, since we only assume that a list of possible causes has been defined (in terms of a set of random variables $\mathrm{\textbf{X}}$) but during the model learning process, the causal relations are autonomously inferred. Note, that the causal models could be used to define the list of preconditions and effects in their action templates. For success prediction, a maximum likelihood estimation is used, which is similar to our approach. Their advantage is that they use success priors for objects that have a similar parent class to preinitialize the action effect, and adapt the prediction based on additional experience. this makes this approach more sample efficient. However, this might not really be applicable for the first problem of cubes, mainly because this appraoch depends greatly on how similar ojects are. Image we define an ontology class shapes which incorporates children like, cube, sphere, pyramid, etc.. It is questionaly if a sphere and a cube have similar success chances for the example of stacking two objects on top of each other. The other problem is precisly because no features are defined and used for predicting action effects, it is not possible to build explanation models on top of it in a similar way as we do. In this sense our approach is required to incorporate more low level information/variables, e.g. the x/y-offset, in order to generate failure explanations. So to summarize, while their method incorporates action effect predictions similar to our appraoch, they do not incorporate object/action features to condition on, which does not allow to generate failure explanations, but only success prediction.
}

\textcolor{blue}{\cite{Das21} presents an approach for generating verbal failure explanations. Their approach requires the definition of a fault tree which defines Failure representation (Fault trees + encoder-decoder network): Failure causes are presented within the framework of \textit{Fault Trees}. Fault trees break down a failure into Failure types (like Navigation, arm motion planning or object detection), which each can have several potential failure causes (e.g. mislocilization or controller error) and can occur during an action like move, segment or grasp. The train an encoder-decoder model which takes as input the current environment state during action execution and outputs a sequence of words that describe the action (which they call $\mathcal{E}_{\pi}$, in case of succesfull execution, or $\mathcal{E}_{err}$ in case of failure at the current state).  
While they claim that their model is white box- in the end, they learn a black-box model that maps states to previously defined and annotated failures. It would be possible to adapt their method to match the error descriptions that we tackle, e.g. by annotating all the potential failures, like 'cube was dropped too far to the right' etc., but then we would need to collect annotated data for many different failure cases. We learn a model that encorporates and generates the failure descriptions only from annotations about the general success of an action. However, we currently have not employed a model that autonomously maps the contrastive state explanations (e.g. x1 instead of x3) to spoken words. Additionally, they do not include an action success prediction. They learn a model that maps a state vector to a particular failure descriptions. They would require labeled execution parameters with labels of the potentially expected failures. In some sense this is a different concept than ours.}

\textcolor{blue}{In~\cite{Das21b}, the same authors propose an alternative approach to generate explanations. They utilize the state-of-the-art scene graph model MOTIFNET~\cite{Zellers18} to predict spatial relationships and object attributes in a given scene, since they were shown to provide more meaningful explanations than their Context-Based History approach in~\cite{Das21}. These semantic information incorporate spatial relations between objects and additional object features like fragile, slippery or hazardous. Among all detected relations that concern the object of interest (e.g. if we want to pick up a bottle, the object of interest is the bottle), the most relevant relations are picked through pairwise ranking. Applying this method to the cube stacking or sphere dropping case would not work, because we consider continuous features (e.g. object was dropped to far to the right or parameters like size are scenario dependent instead of simple object features) as potential failure causes (although MOTIFNET could be used to autonomously detect the action outcome). Also their approach mentions many environment relations which are not necessarily contributing to generating a failure. They do not incorporate any failure predication but base the choice of relation on training a random forest classifier that ranks potential problems.}

\textcolor{blue}{This might be an interesting approach to find a better explanations in our case as well, however this would require additional domain knowledge from the user. Our current approach is based on the assumptions that the simplest solution is the best~\cite{Miller19Explanation} (Occams Razor). In our case that means, we want as few interval changes as possible. This does not necessarily mean that this is always and under all circumstances the most informative or intuitive explanations from a human perspective. However, without any additional domain knowledge, provided by humans, this seems to be one of the most intuitive solutions. In future work, we could acquire additional input from humans and incorporate it in form of search heuristics (e.g., to punish changes for specific variables like in the sphere dropping case, we might want to avoid changing the container, so we first look for a solution in the x/y-Offset variables.}

have a very similar objective but propose 
Two works that come close in terms of generating failure explanations are~\cite{Das21, Das21b}. In~\cite{Das21} they find out that Context-based explanations that include the action history (current action, previous action and cause of failure) are most informative for humans. Then they learn a encoder-decoder network that maps the current environment state to a verbal failure explanation. The disadvantage of this appraoch is that while they claim to work on explainable robotics, in the end learn a black-box mapping to explanations of the current state. Another problem is that they require labeled simulations for each potential failure case. Out model inherently captures all possible failures in one model. Also the failures need to be hand-defined, while we learn them, thus learning a causal understanding of the environemnt (more flexibility, less assumed knowledge).
In a follow up~\cite{Das21b}, the authors use a semantic scene analyser to automatically retrieve geometric relations between objects (like above  and below) and object features (like heavy) from images. Then they present a method that generates failure explanations for pick and place actions. The trick is that they leverage pairwise ranking to filter out the most meaningful spatial relations that are most likely the cause of the failure. But again they do not incorporate a probabilistic predication framework as we do to predict the most likely causes for a failure. Plus, since it is mainly based on spatial features, it cannot explain failures that we tackle in our work like 'the cube was stacked too far too the left.' 
\textbf{TODO: add Vasumathi and Hasas: explaining impossble high-level robot behaviors.}

% \vspace{-5mm}
% \small
% \begin{equation}
% \begin{split}
% \text{sim2real} &= \frac{1}{|\texttt{xOff}_{\text{e}}| |\texttt{yOff}_{\text{e}}| |\texttt{dropOff}_{\text{e1}}|}
%                  \sum_{x=1}^{|\texttt{xOff}_{\text{e}}|}\sum_{y=1}^{|\texttt{yOff}_{\text{e}}|}\sum_{d=1}^{|\texttt{dropOff}_{\text{e1}}|}  \\
%                 &\bigg( 1 - \Big(\big|P_{real}(\texttt{onTop}=1 |\texttt{xOff}_{\text{e}}=x, \texttt{yOff}_{\text{e}}=y,
%                 \\
%                 & \; \; \; \; \; \; \texttt{dropOff}_{\text{e1}}=d) - P_{sim}(\texttt{onTop}=1 |\texttt{xOff}=x, \\
%                 & \; \; \; \; \; \; \texttt{yOff}=y, \texttt{dropOff}=d) \big| \Big) \bigg)
% \end{split}
% \end{equation}
% \normalsize
\begin{table}[]
\begin{tabular}{|l|l|l|l|}
\hline
Method & 
CB-H~\cite{Das21} & 
SSG-R~\cite{Das21b} & 
ours \\
\hline
\hline
\begin{tabular}[c]{@{}l@{}}Idea\end{tabular}& 
\begin{tabular}[c]{@{}l@{}} Fault trees +\\encoder-decoder \\network\end{tabular} & 
\begin{tabular}[c]{@{}l@{}}\begin{tabular}[c]{@{}l@{}} MOTIFNET~\cite{Zellers18} + \\pairwise ranking\end{tabular}\end{tabular} & 
\begin{tabular}[c]{@{}l@{}}causal BNs\\+ contrastive\\BFS \end{tabular} \\
\hline
\begin{tabular}[c]{@{}l@{}}Input\end{tabular} & 
\begin{tabular}[c]{@{}l@{}}robot and obj. \\states (positions,\\ velocities, object/\\robot trans-\\formations)\end{tabular} & 
\begin{tabular}[c]{@{}l@{}}images\end{tabular} & 
\begin{tabular}[c]{@{}l@{}}Parametri-\\zation\\of $\mathrm{\textbf{X}}$\end{tabular}\\
\hline
\begin{tabular}[c]{@{}l@{}}Output\end{tabular} & 
\begin{tabular}[c]{@{}l@{}}language model\\spoken failure\\explanation\end{tabular} &
\begin{tabular}[c]{@{}l@{}}explanation with\\relevant spatial and\\object relations\end{tabular} & 
\begin{tabular}[c]{@{}l@{}}contrastive\\failure\\explanation\end{tabular}\\
\hline
\begin{tabular}[c]{@{}l@{}}Learning\\Prerequi-\\sites\end{tabular} & 
\begin{tabular}[c]{@{}l@{}}failure-cause\\annotated\\simulations\end{tabular} & 
\begin{tabular}[c]{@{}l@{}}relationship\\ranking\\labels\end{tabular} & 
\begin{tabular}[c]{@{}l@{}}samples $d$\\(incl. action\\outcome)\end{tabular}\\
\hline
\begin{tabular}[c]{@{}l@{}}Action\\Succ.\\Prediction\end{tabular} & no & no & \begin{tabular}[c]{@{}l@{}}MLE (or sim-\\ilar like\\Bayesian  est.)\end{tabular}\\
\hline
\end{tabular}
\caption{\textcolor{blue}{Comparison of our explanation generation pipeline with other approaches.}}
\label{tab:baseline}
\end{table}

\begin{table*}[]
\begin{tabular}{|l|l|l|l|l|l|}
\hline
Method & 
\begin{tabular}[c]{@{}l@{}}Idea\end{tabular} & 
Output & 
Input & 
\begin{tabular}[c]{@{}l@{}}(Learning)\\ 
Prerequisites\end{tabular} & 
Action Succ. Prediction   \\
\hline
\hline
\begin{tabular}[c]{@{}l@{}}CB-H\\\cite{Das21}\end{tabular}& 
\begin{tabular}[c]{@{}l@{}} Fault trees \\+ encoder-\\decoder \\network\end{tabular} & 
\begin{tabular}[c]{@{}l@{}}language model/\\ spoken failure \\ explanation\end{tabular} & 
\begin{tabular}[c]{@{}l@{}}robot and obj. states\\ (positions, velocities, \\ object/robot transfor-\\mations (relations))\end{tabular} & 
\begin{tabular}[c]{@{}l@{}}  failure-cause \\ annotated \\ simulations\end{tabular} & 
\begin{tabular}[c]{@{}l@{}}no\end{tabular}                                                              \\
\hline
\begin{tabular}[c]{@{}l@{}}SSG-R\\\cite{Das21b}\end{tabular}& 
\begin{tabular}[c]{@{}l@{}} MOTIFNET~\cite{Zellers18} + \\pairwise ranking\end{tabular} & 
\begin{tabular}[c]{@{}l@{}}explanation with \\relevant spatial and \\object relations\end{tabular} & 
\begin{tabular}[c]{@{}l@{}}images\end{tabular} & 
\begin{tabular}[c]{@{}l@{}} relationship \\ranking \\labels\end{tabular} & 
\begin{tabular}[c]{@{}l@{}}no\end{tabular} \\
% \hline
% Bauer et al. & 
% Planning Operators & 
% \begin{tabular}[c]{@{}l@{}}action success \\prediction \end{tabular}& 
% \begin{tabular}[c]{@{}l@{}}predefined high level action \\ description (precondition \\and effects)\end{tabular} & 
% & 
% MLE & 
% no                                                                           \\
\hline
ours & 
\begin{tabular}[c]{@{}l@{}}causal BNs +\\contrastive BFS \end{tabular}& 
\begin{tabular}[c]{@{}l@{}}contrastive failure \\explanation \end{tabular}& 
\begin{tabular}[c]{@{}l@{}}parametrization of $\mathrm{\textbf{X}}$ \end{tabular}& 
\begin{tabular}[c]{@{}l@{}}samples $d$ \\
(including action \\
outcome)\end{tabular}& 
\begin{tabular}[c]{@{}l@{}}MLE (or similar estimators \\ like Bayesian estimator)\end{tabular} \\
\hline
\end{tabular}
\caption{Comparison of our explanation generation pipeline with other approaches.}
\label{tab:baseline}
\end{table*}

\begin{table*}[]
\begin{tabular}{|l|l|l|l|l|l|}
\hline
 & 
\begin{tabular}[c]{@{}l@{}}Method\end{tabular} & 
Output & 
Input & 
\begin{tabular}[c]{@{}l@{}}Learning  
Prerequisites\end{tabular} & 
Task Succ. Predict.   \\
\hline
\hline
\begin{tabular}[c]{@{}l@{}}CB-H\\\cite{Das21}\end{tabular}& 
\begin{tabular}[c]{@{}l@{}} Fault trees + encoder-\\decoder network\end{tabular} & 
\begin{tabular}[c]{@{}l@{}}language model/ spoken \\ failure explanation\end{tabular} & 
\begin{tabular}[c]{@{}l@{}}robot and obj. states (positions, \\velocities, object/robot relations)\end{tabular} & 
\begin{tabular}[c]{@{}l@{}}  failure-cause annotated \\ simulations\end{tabular} & 
\begin{tabular}[c]{@{}l@{}}no\end{tabular}                                                              \\
\hline
\begin{tabular}[c]{@{}l@{}}SSG-R\\\cite{Das21b}\end{tabular}& 
\begin{tabular}[c]{@{}l@{}} MOTIFNET~\cite{Zellers18}\\+ pairwise ranking\end{tabular} & 
\begin{tabular}[c]{@{}l@{}}list of relevant \\ spatial and object relations\end{tabular} & 
\begin{tabular}[c]{@{}l@{}}images\end{tabular} & 
\begin{tabular}[c]{@{}l@{}}relationship ranking \\labels\end{tabular} & 
\begin{tabular}[c]{@{}l@{}}no\end{tabular} \\
\hline
ours & 
\begin{tabular}[c]{@{}l@{}}causal BNs +\\contrastive BFS \end{tabular}& 
\begin{tabular}[c]{@{}l@{}}contrastive failure \\variable parametrizations \end{tabular}& 
\begin{tabular}[c]{@{}l@{}}parametrization of $\mathrm{\textbf{X}}$ \end{tabular}& 
\begin{tabular}[c]{@{}l@{}}samples $d$ (including \\action
outcome)\end{tabular}& 
\begin{tabular}[c]{@{}l@{}}MLE (or similar \\ like Bayesian est.)\end{tabular} \\
\hline
\end{tabular}
\caption{Comparison of our explanation generation pipeline with other approaches.}
\label{tab:baseline}
\end{table*}
